# Supplementary material for: Mobility Data in Operations: The Facility Location Problem
Source: arXiv:2301.06246 source file (2023-12-10)
Supplement: Supplementary file 1 [file apx-scaledcostapprox.tex]

\scaledcostapprox*

\begin{proof}
    Fix an arbitrary instance $\instance$, 
    we can upperbound the total cost of $\ALG$ on instance $\instance$ as follows,
    \begin{align*}
        \Cost{\ALG(\instance)} = 
    \end{align*}

    For every instance $\instance = (n, \distance, 
\{\flowe\}_{\edge\in\Edge}, \opencosts_{i\in[n]})$, construct a modified instance $\instance\primed = (n, \distance, 
\{\flowe\}_{\edge\in\Edge}, \opencosts\primed_{i\in[n]})$ with modified facility opening cost $\opencosti\primed = \costscalar\cdot \opencosti$. 
    Namely, the modified instance $\instance\primed$ is the same as the original instance $\instance$, except that its facility opening costs are scaled up by a multiplicative factor of $\costscalar$ from the original instance.
    We can upperbound the total cost of $\ALG$ on instance $\instance$ as follows,
    \begin{align*}
        \Cost{\ALG(\instance)} =
        \Cost{\ALG(\instance)}
    \end{align*}

    Let $\SOL = \ALG(\instance\primed)$ be the solution returned by algorithm $\ALG$ for the modified instance $\instance\primed$,
    and $\OPT$ be the optimal solution for instance $\instance$.
    Note that 
    \begin{align*}
        \Cost[\instance]{\widetilde{\ALG}}
        &=
        \CostF[\instance]{\SOL}
        +
        \CostC[\instance]{\SOL}
        \\
        &\overset{(a)}{=} 
        \frac{1}{\costscalar}\CostF[\instance\primed]{{\SOL}}
        +
        \CostC[\instance\primed]{{\SOL}}
        \\
        &\overset{(b)}{\geq} 
        \approxratio\cdot 
        \left(
        \frac{1}{\costscalar}\CostF[\instance\primed]{{\OPT}}
        +
        \CostC[\instance\primed]{{\OPT}}
        \right)
        \\
        &\overset{(c)}{=}  
        \approxratio\cdot 
        \left(
        \CostF[\instance]{\OPT}
        +
        \CostC[\instance]{\OPT}
        \right)
        % \\
        % &
        = 
        \approxratio\cdot 
        \Cost[\instance]{\OPT}
    \end{align*}
    where equalities~(a) (c) holds due to the construction of 
    the modified instance $\instance\primed$,
    and inequality holds due to the assumption of algorithm $\ALG$ in the lemma statement.
\end{proof}
