# Supplementary material for: Mobility Data in Operations: The Facility Location Problem
Source: arXiv:2301.06246 source file (2023-12-10)
Supplement: Supplementary file 2 [file apx-numerical-additional-results.tex]

\section{Additional Results 
for Numerical Experiments}
\label{apx:numerical additional results}

Here we present 
additional numerical results 
of the experiments over synthetic 
data. 
The experimental setup is the same 
as \Cref{sec:numerical synthetic},
except that the cost distribution 
$\texttt{Exponential}(\sfrac{1}{100})$
is replaced with 
$\texttt{Exponential}(\sfrac{1}{50})$
and 
$\texttt{Exponential}(\sfrac{1}{200})$.
In all setups, our observations in \Cref{sec:numerical synthetic} 
preserve. 
Specifically, $\CFAlgP(1)$ outperforms all other policies,
and the performance gap between $\CFAlgP(1)$ and $\GDH$, $\GDW$
is significant.
See the normalized performance for different policies
in \Cref{fig:numerical synthetic ratio ExpDist(1/50)},
\Cref{fig:numerical synthetic ratio ExpDist(1/200)},
\Cref{table:numerical synthetic ratio ExpDist(1/50)}
and \Cref{table:numerical synthetic ratio ExpDist(1/200)}.

\begin{figure}[ht]
  \centering
       \subfloat[uniform $\{\flowi\}$]
      {\includegraphics[width=0.45\textwidth]{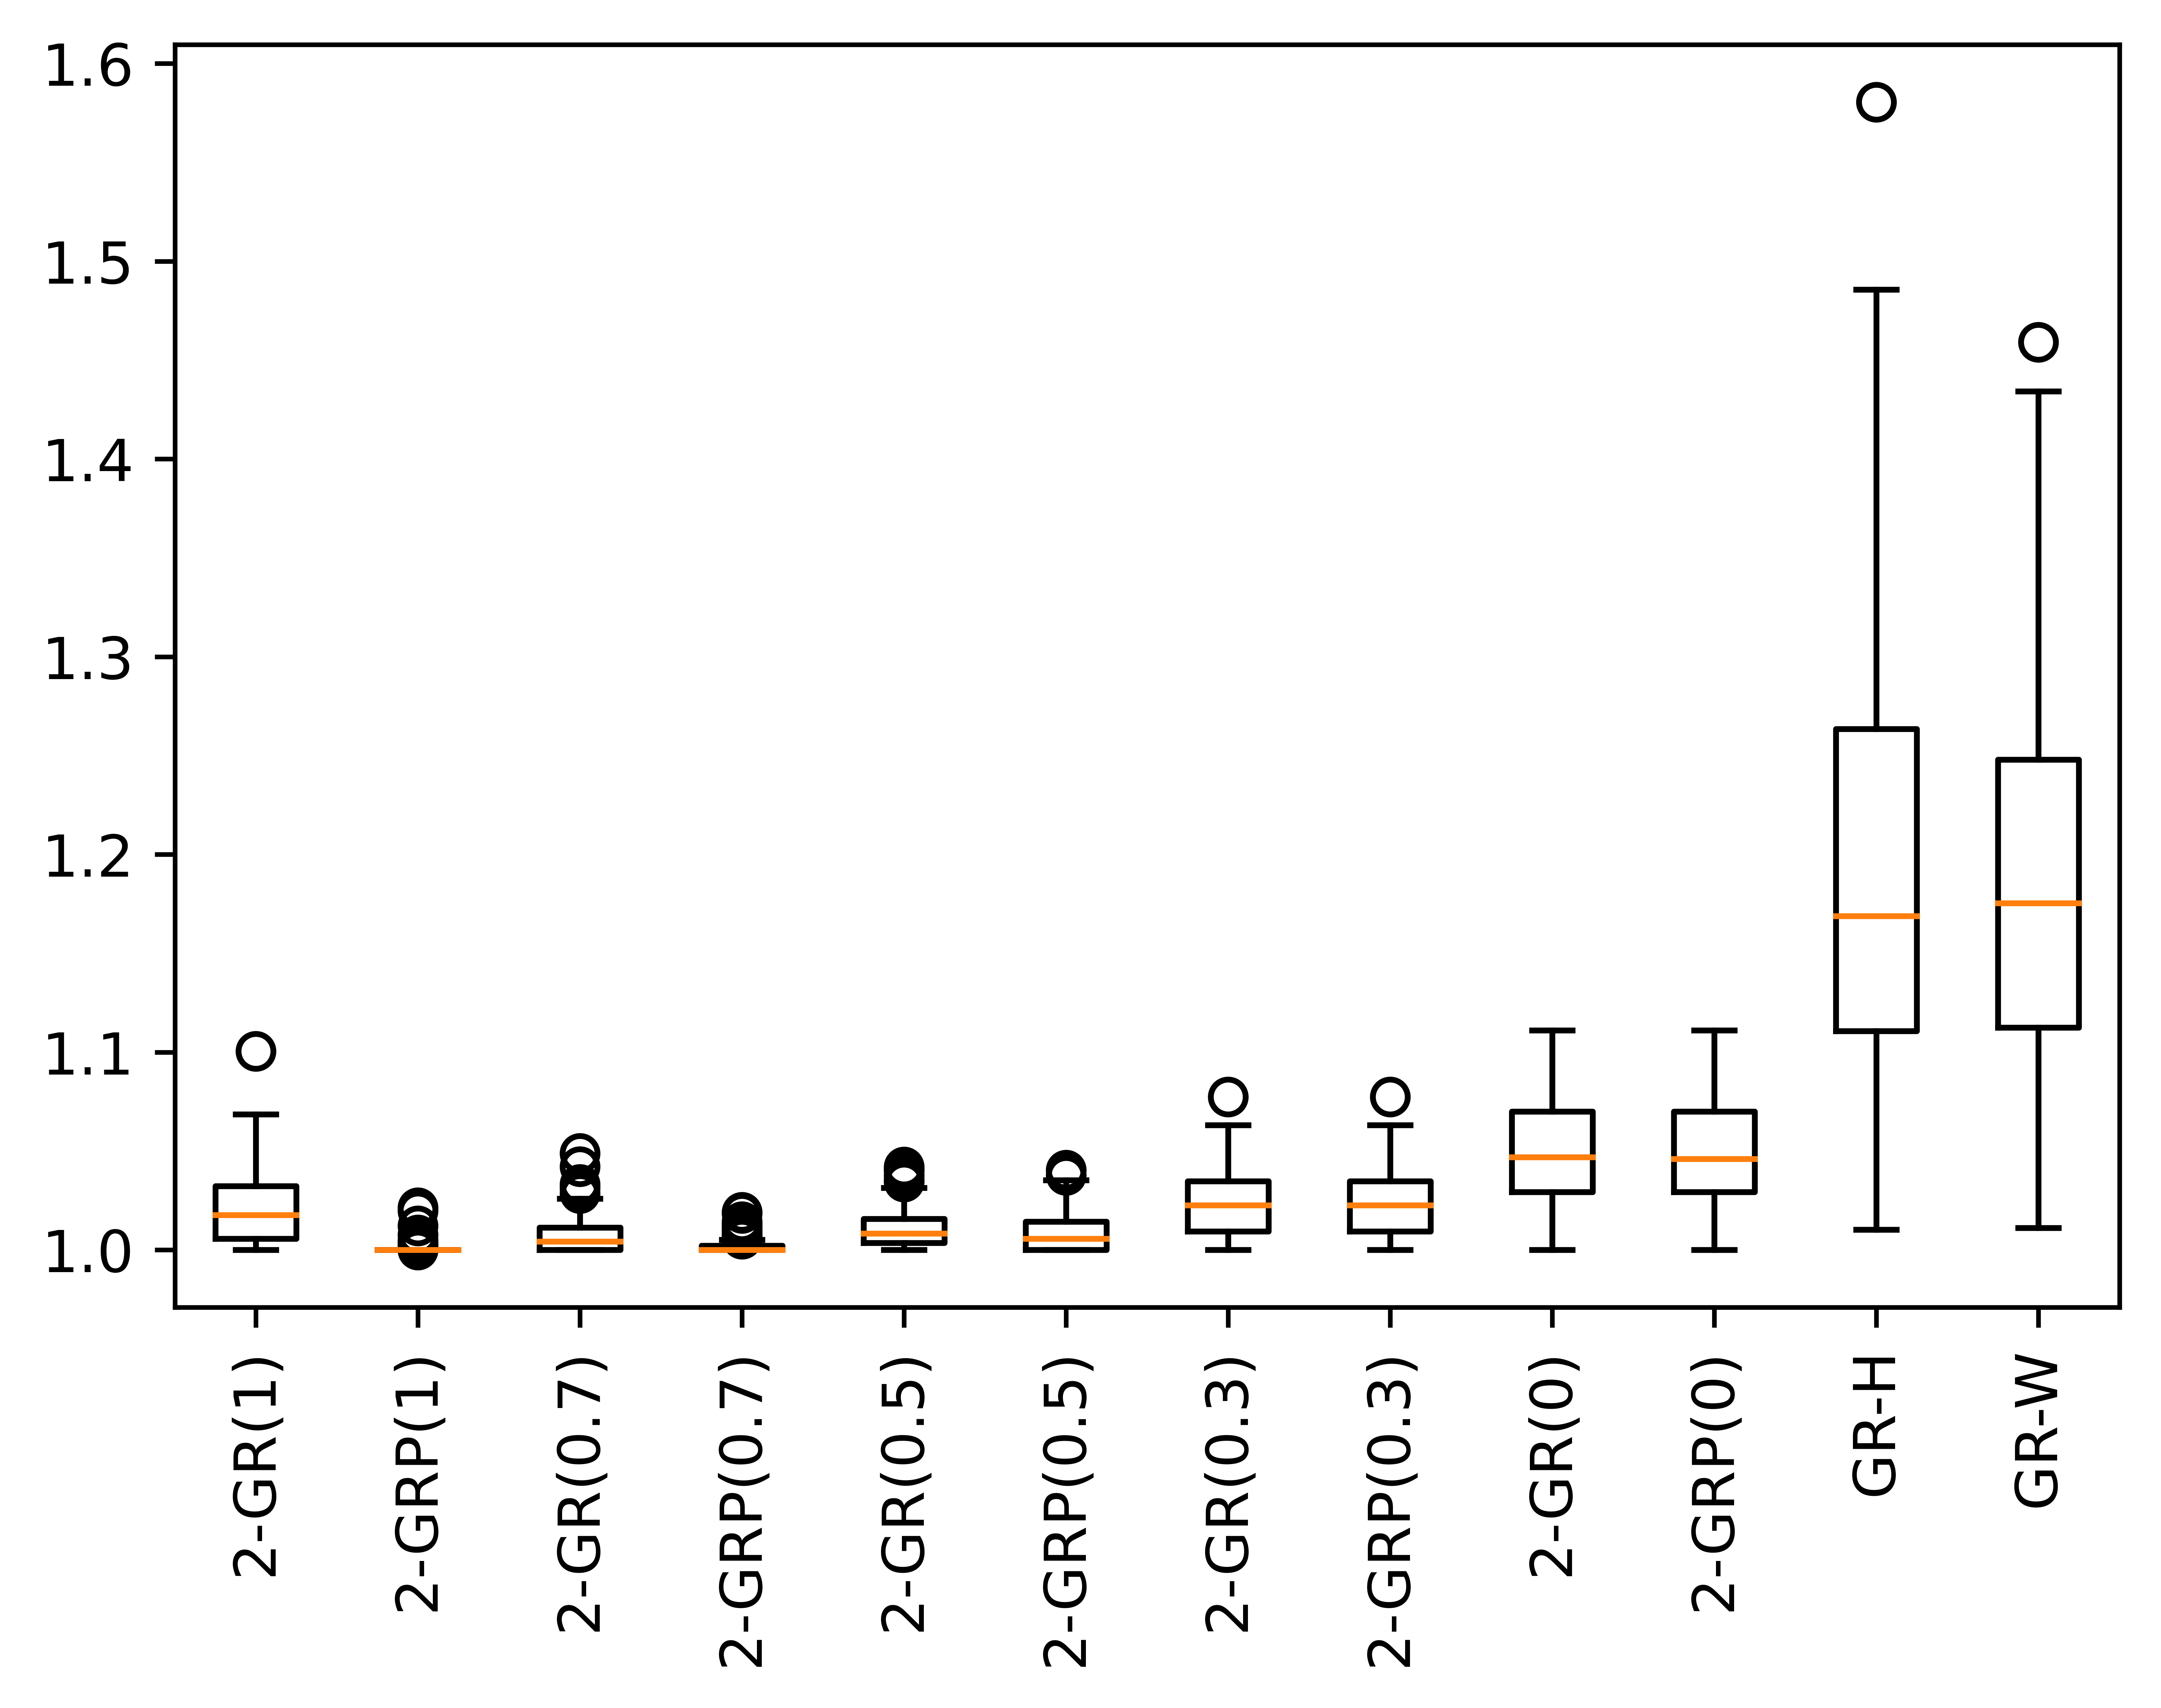}}
      ~~~~
      ~~~~
      \subfloat[distance-discounted $\{\flowi\}$]
      {\includegraphics[width=0.45\textwidth]{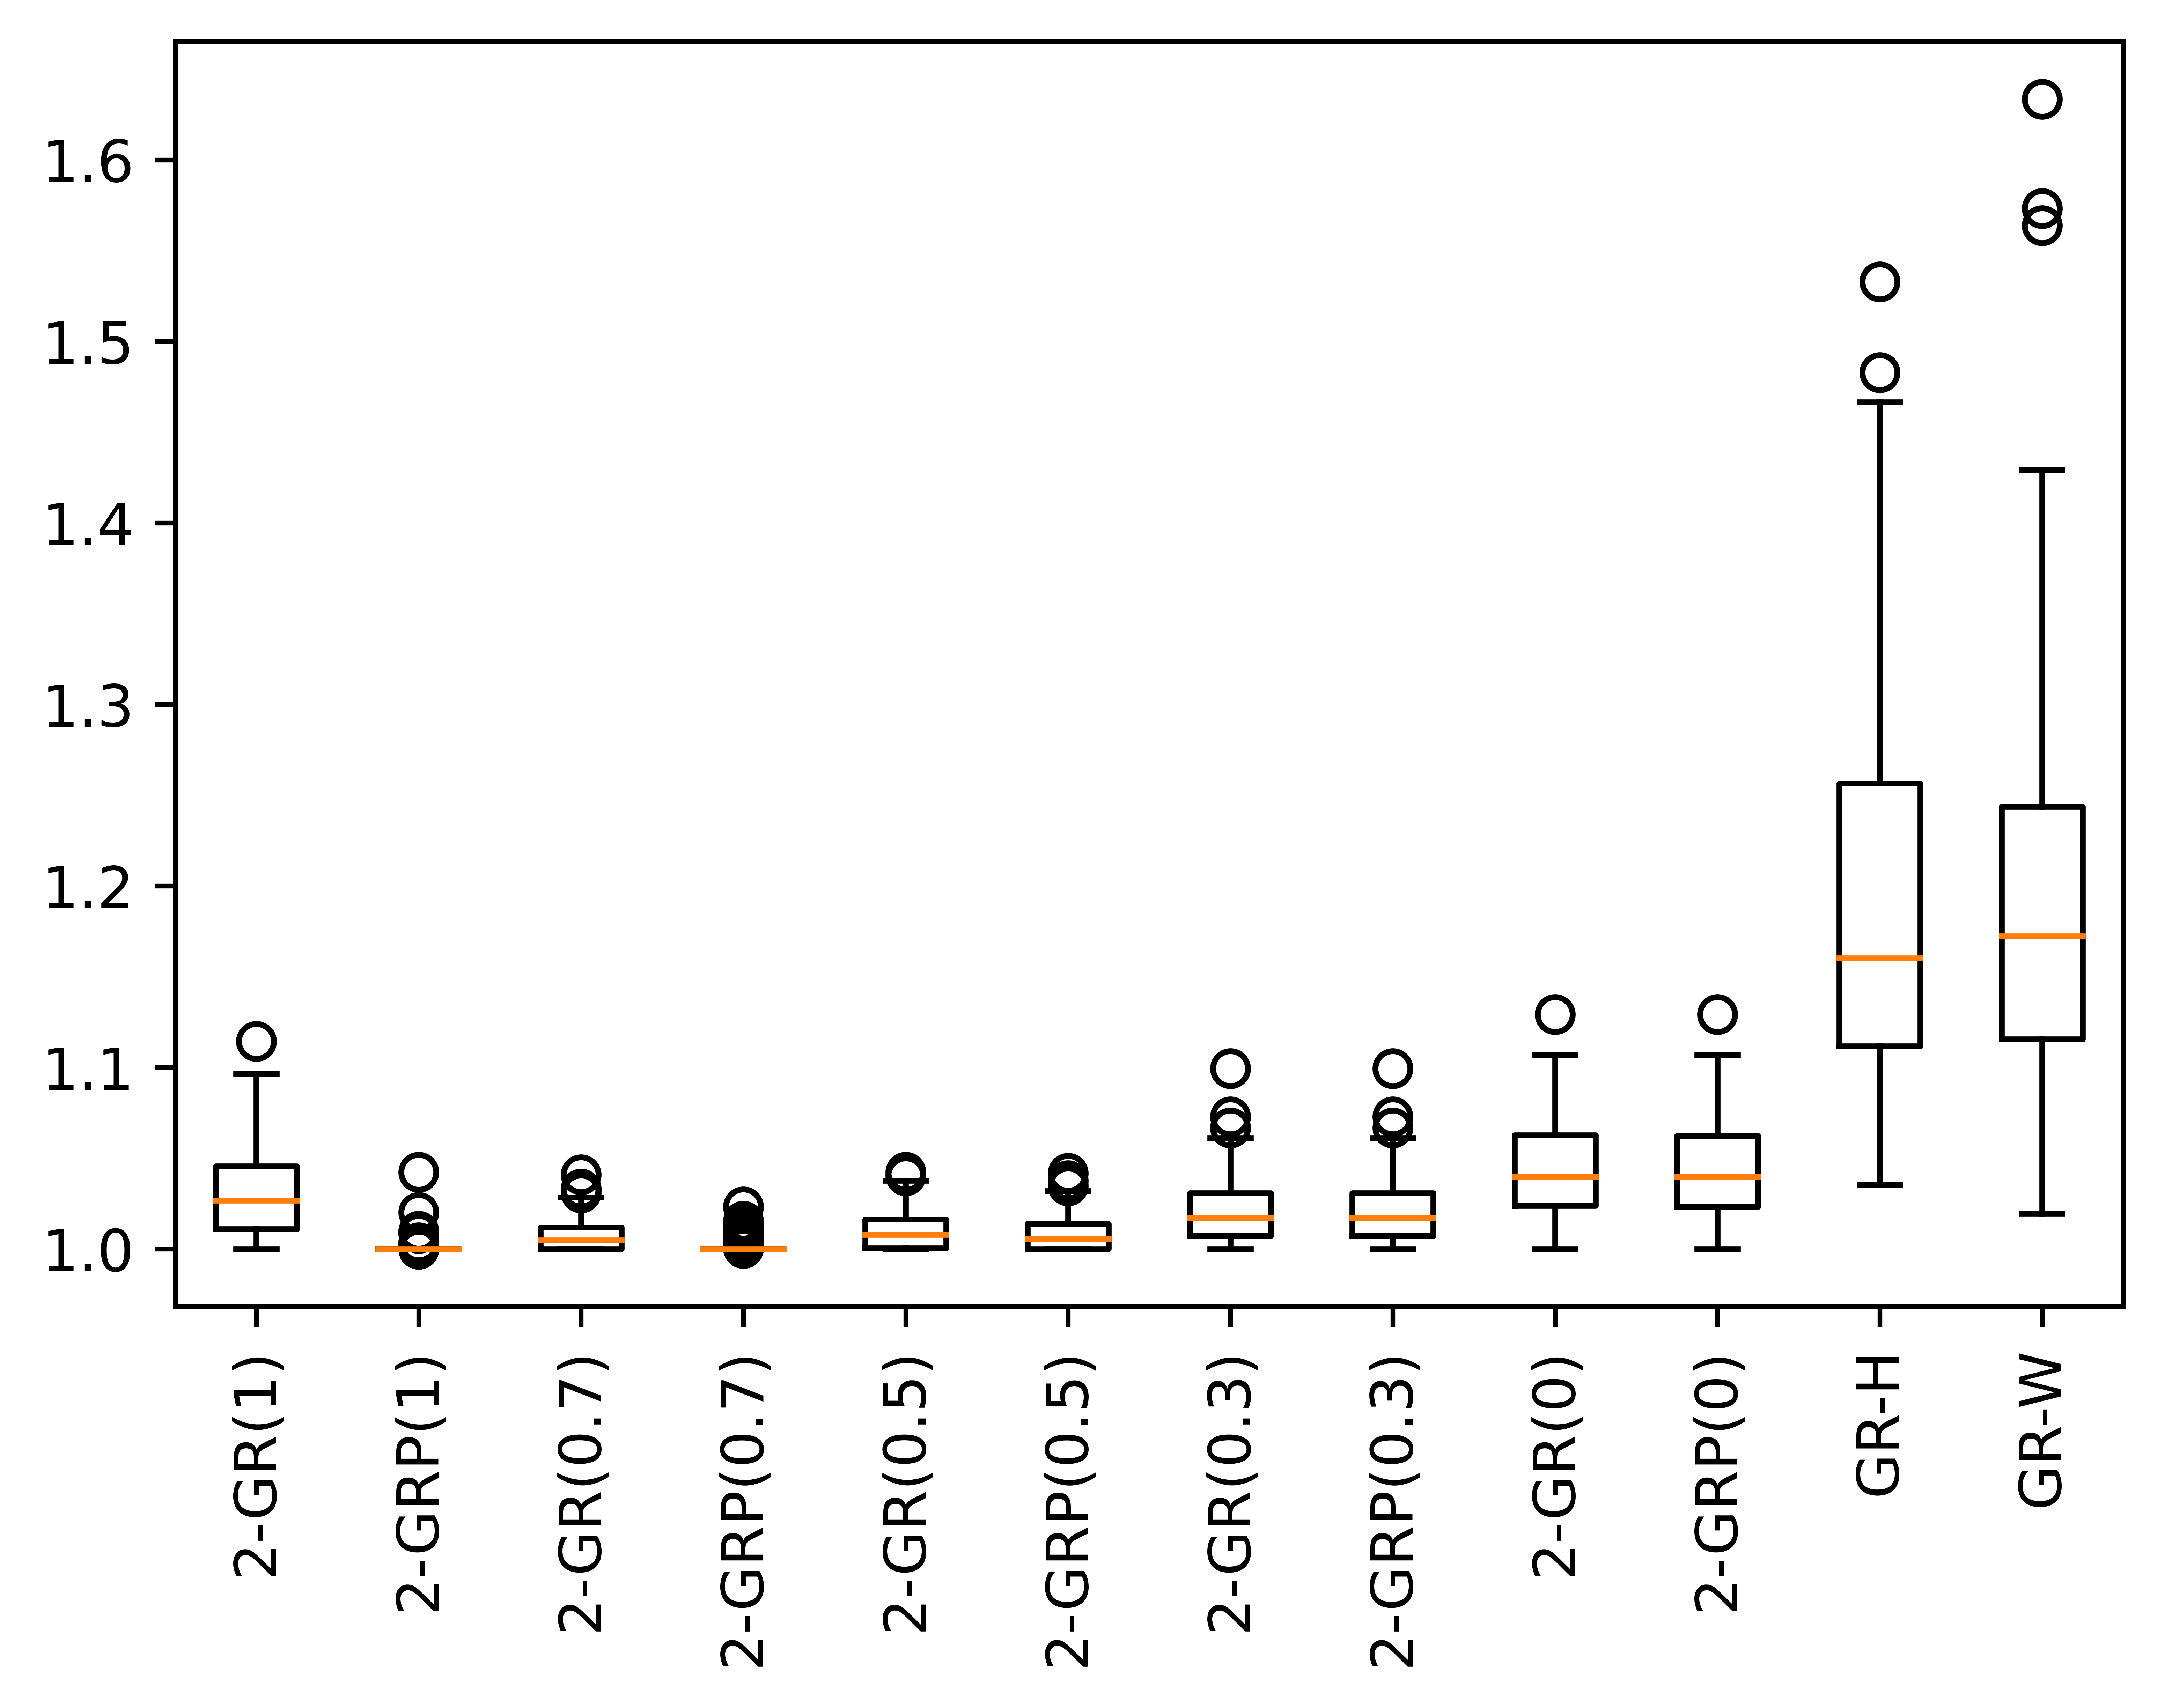}}
  \caption{Comparison of different policies in terms of the normalized performance. Facility opening costs $\{\opencost_i\}$
  are drawn i.i.d.\ from $\texttt{Exponential}(\sfrac{1}{50})$.
  Results are based on 100 i.i.d.\ random instance.
  }
   \label{fig:numerical synthetic ratio ExpDist(1/50)}
\end{figure}

\begin{figure}[ht]
  \centering
       \subfloat[uniform $\{\flowi\}$]
      {\includegraphics[width=0.45\textwidth]{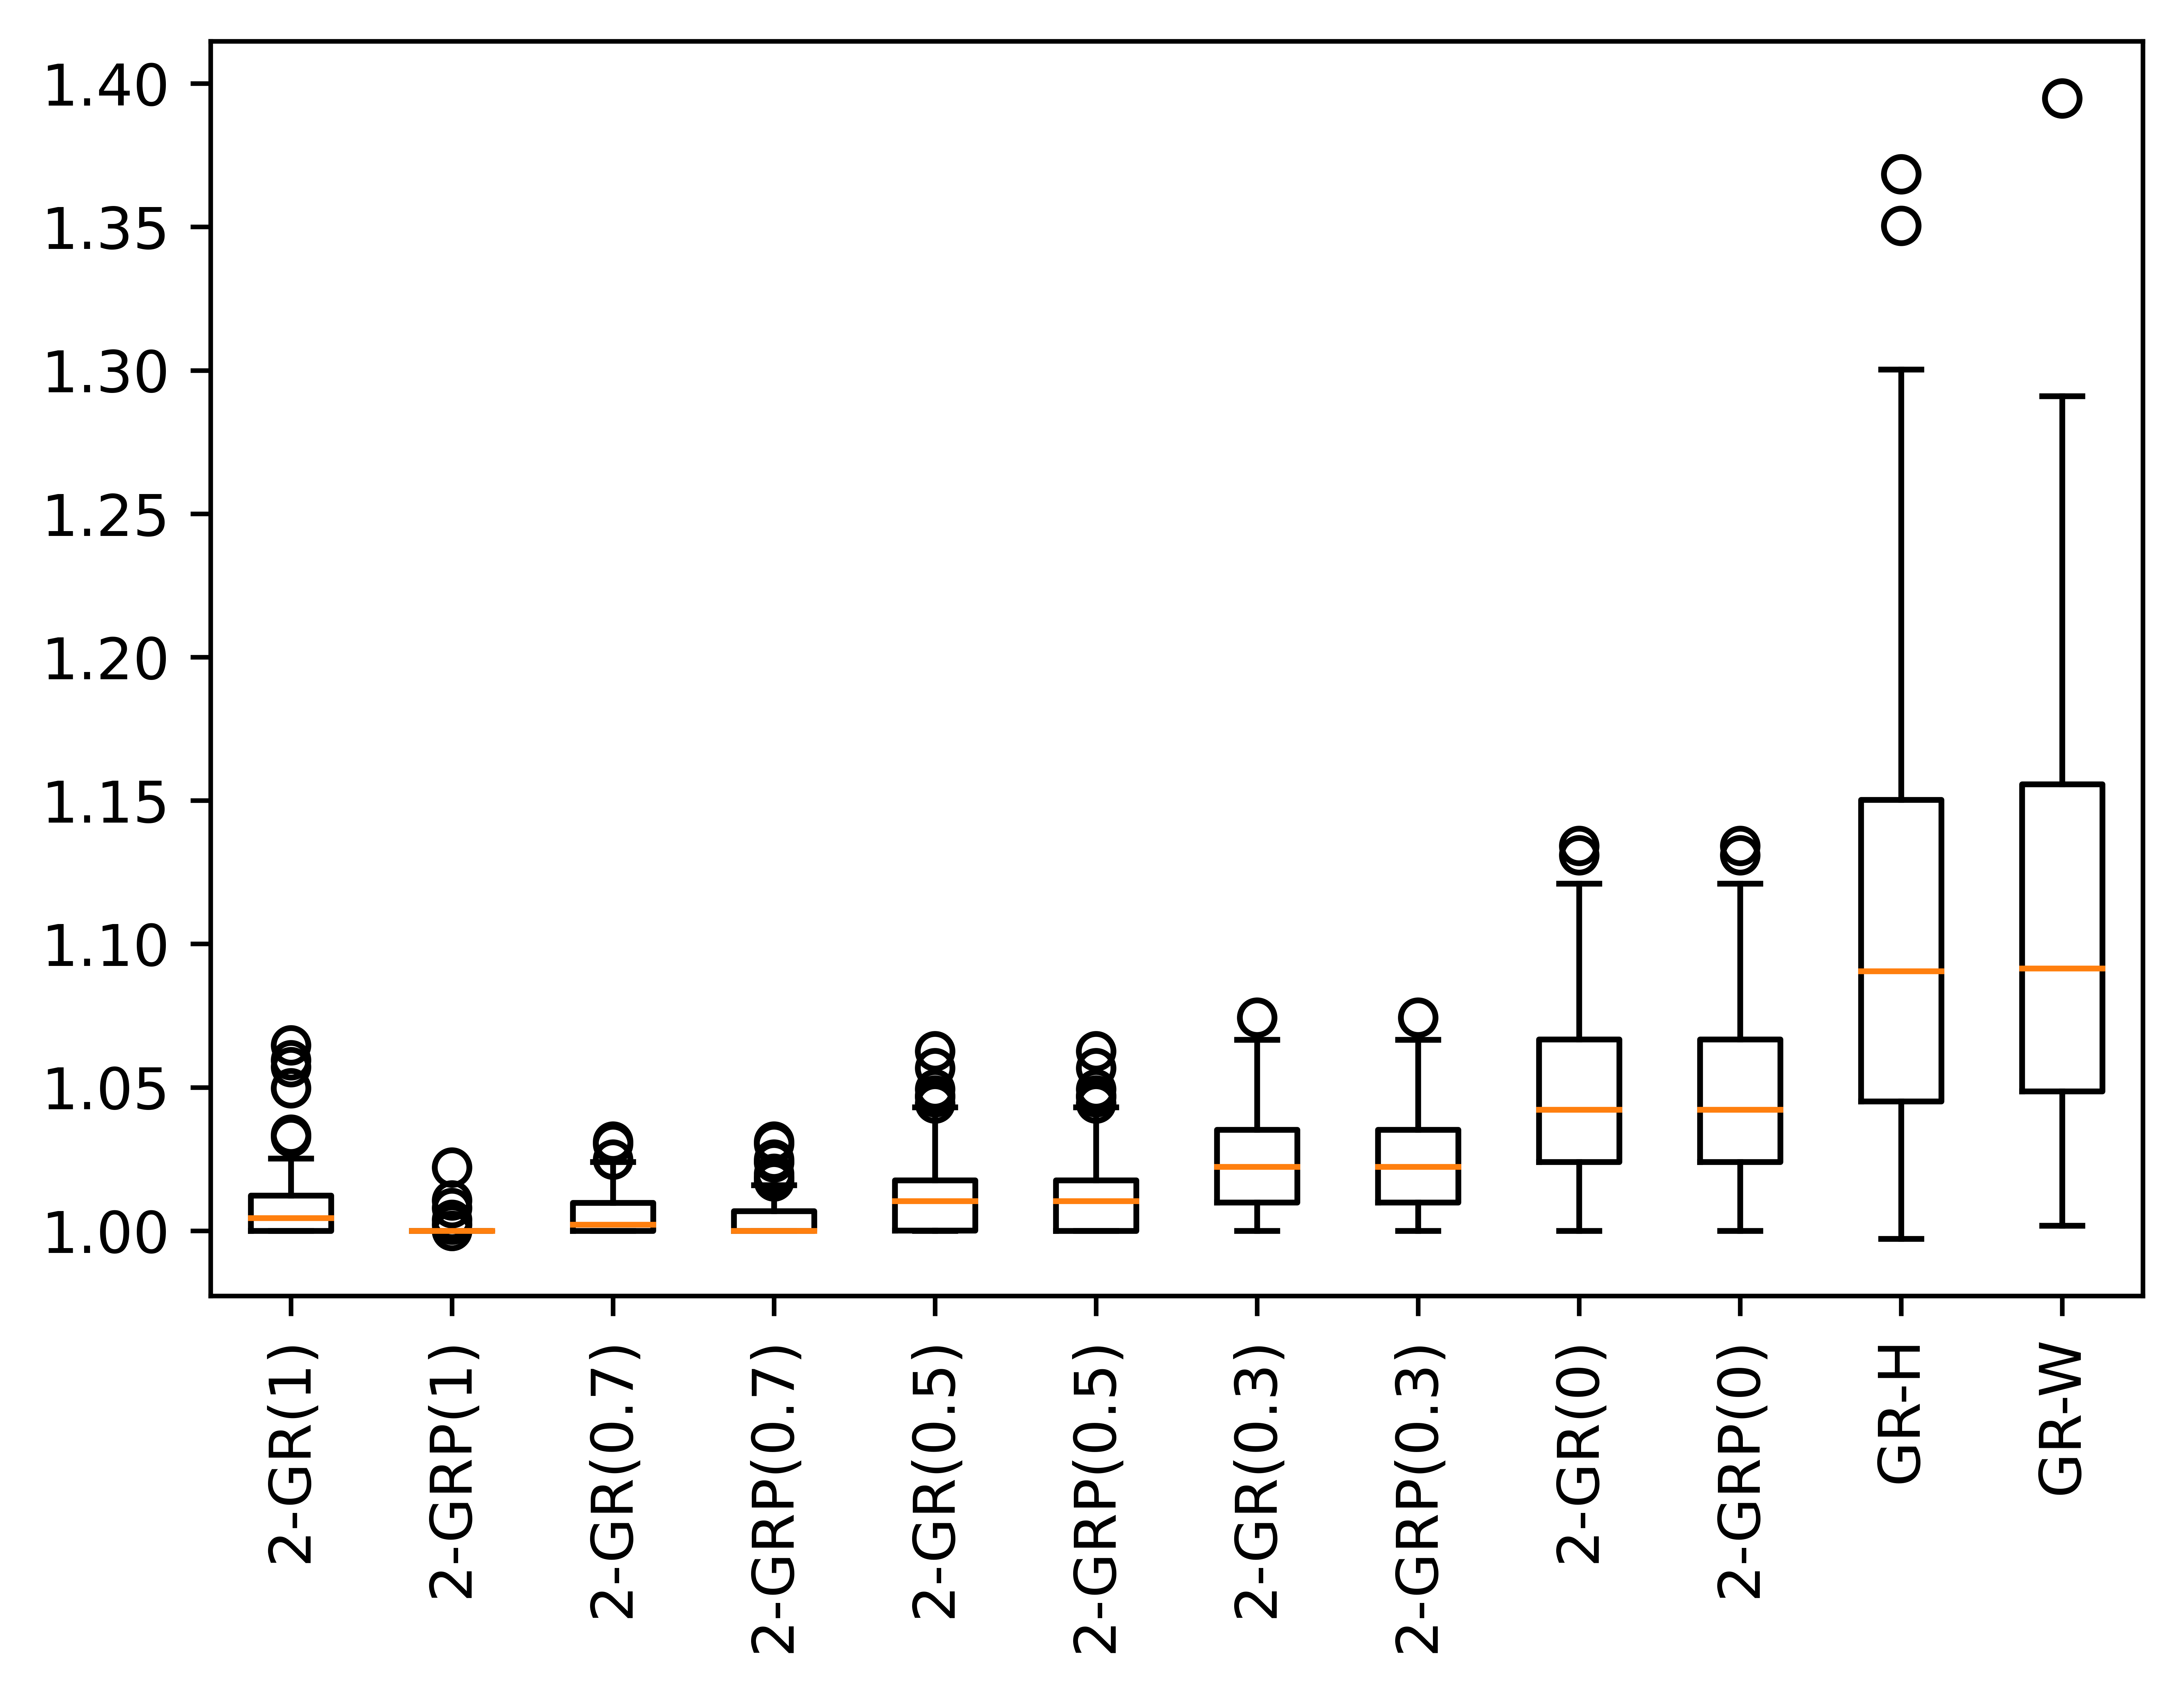}}
      ~~~~
      ~~~~
      \subfloat[distance-discounted $\{\flowi\}$]
      {\includegraphics[width=0.45\textwidth]{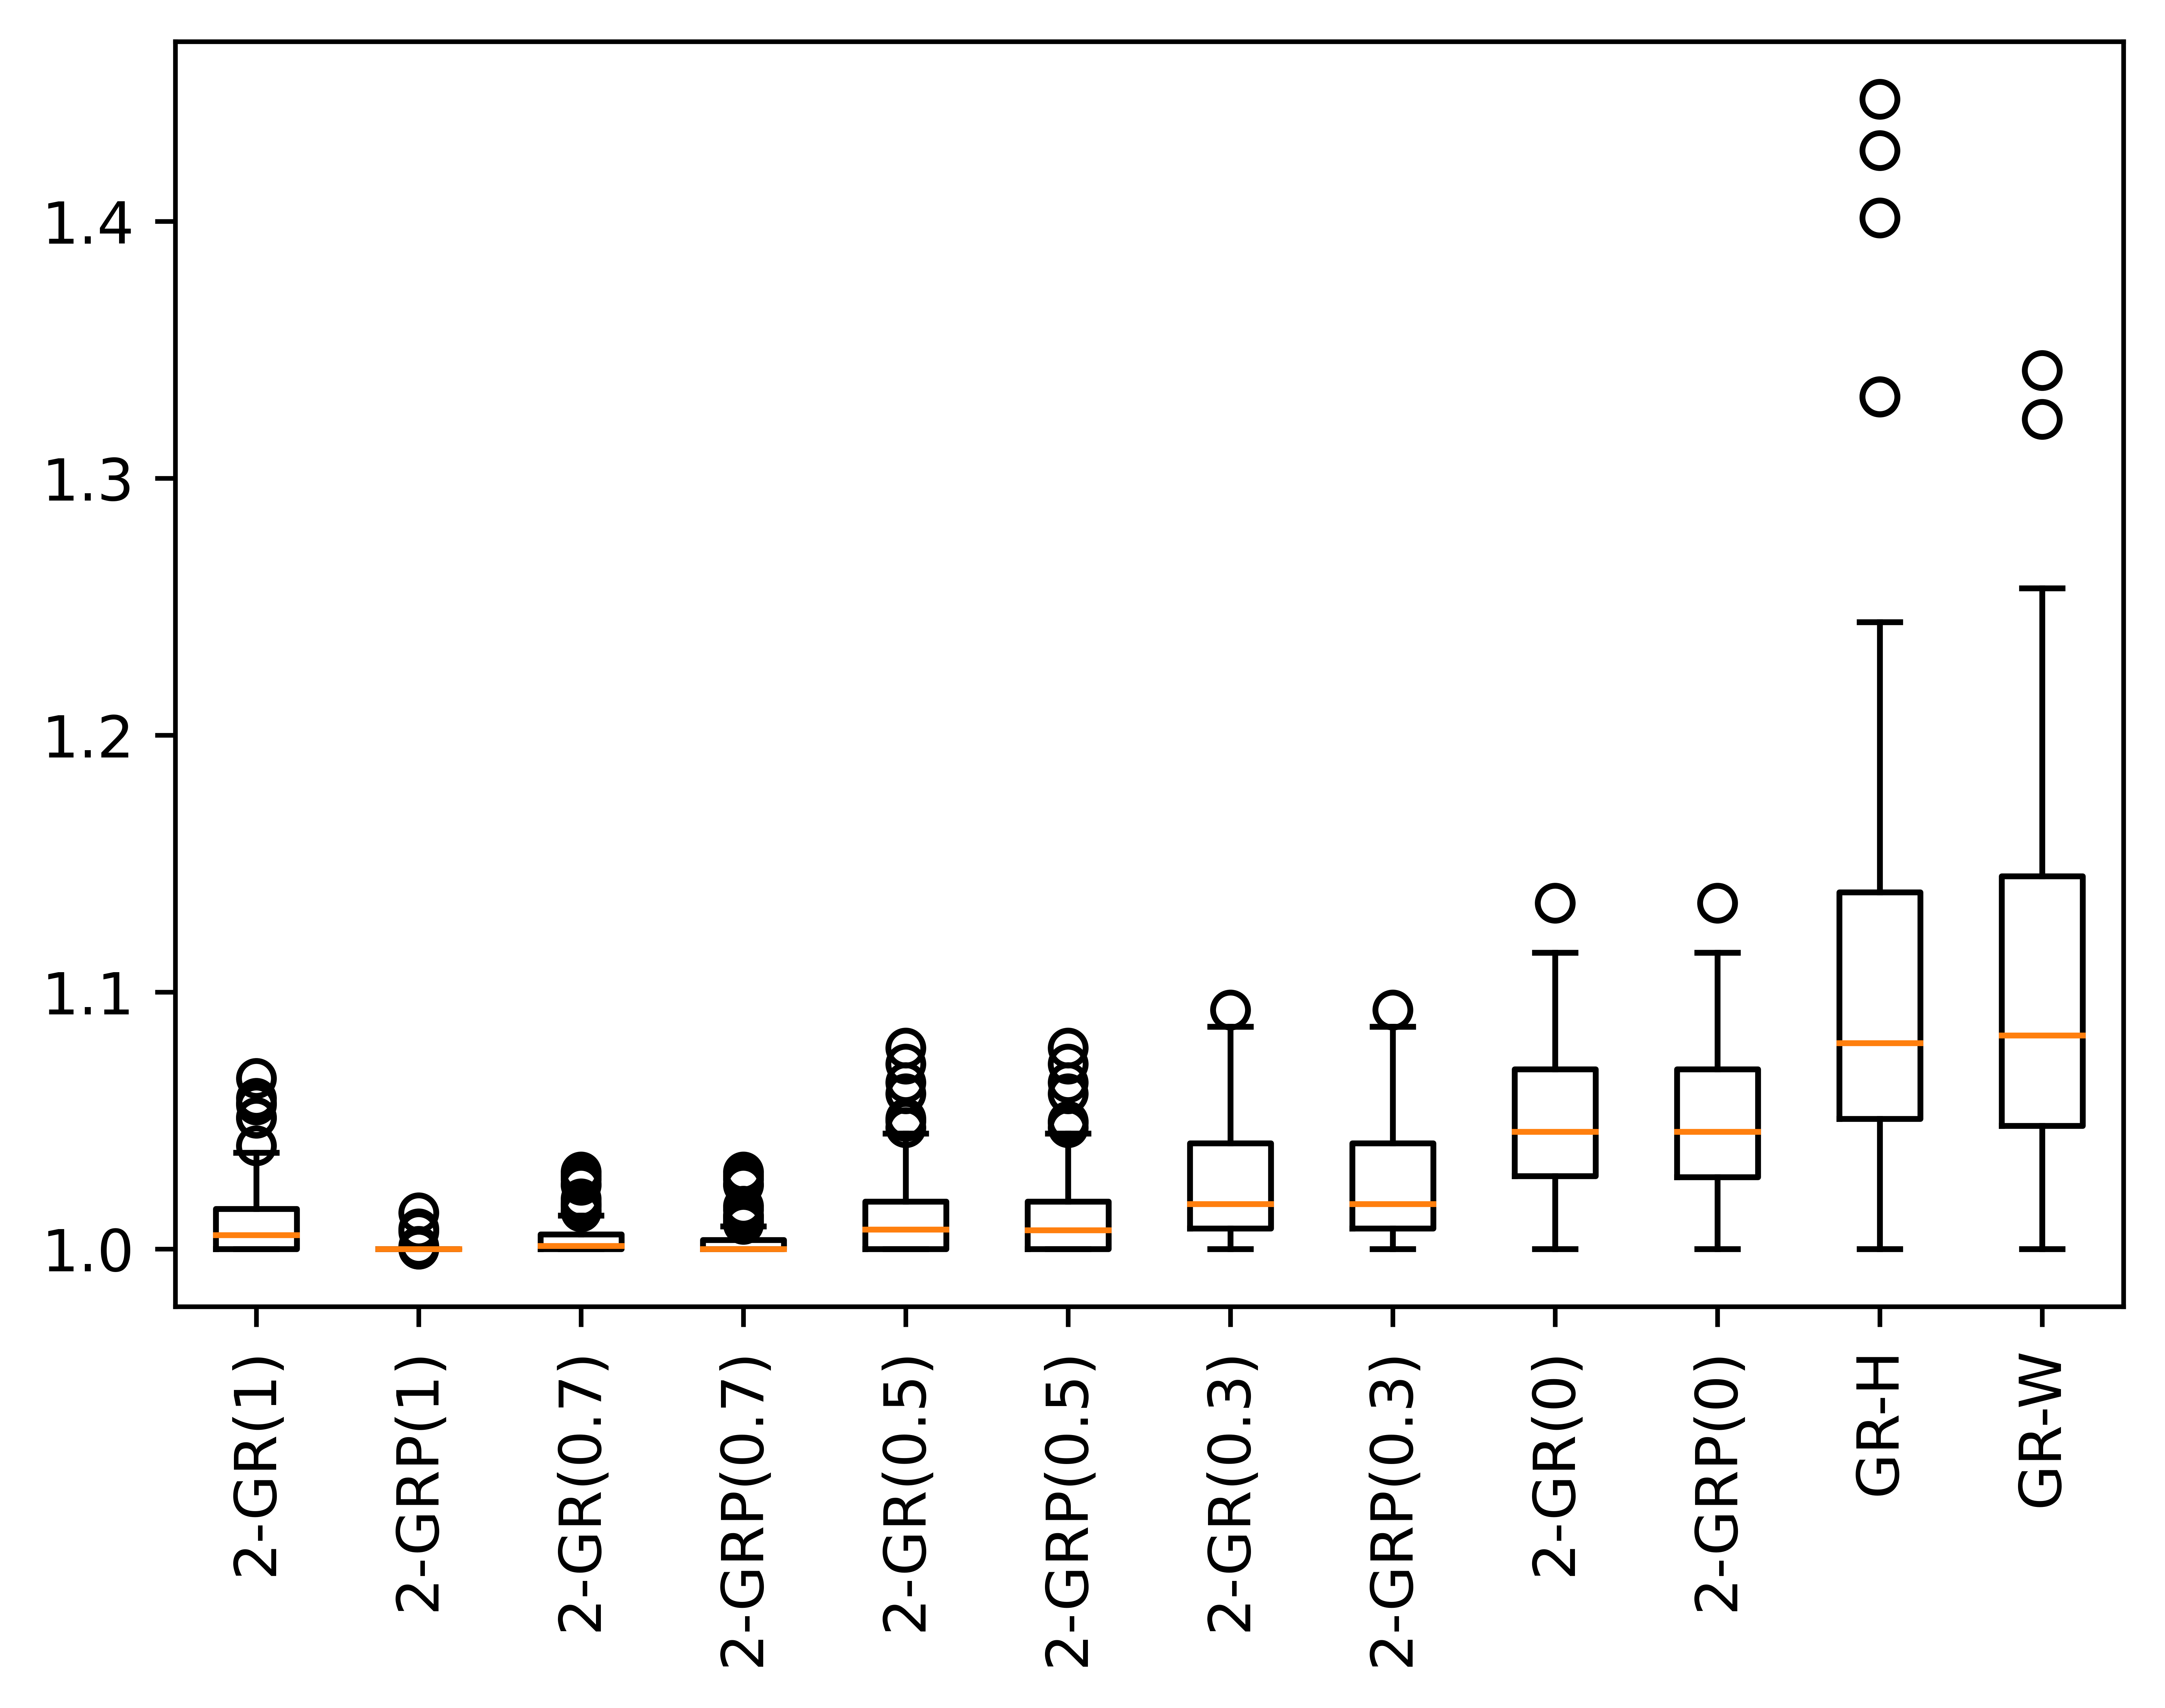}}
  \caption{Comparison of different policies in terms of the normalized performance. Facility opening costs $\{\opencost_i\}$
  are drawn i.i.d.\ from $\texttt{Exponential}(\sfrac{1}{200})$.
  Results are based on 100 i.i.d.\ random instance.
  }
   \label{fig:numerical synthetic ratio ExpDist(1/200)}
\end{figure}

\begin{table}[ht]
    \centering
    \caption{The average normalized performance for 
    different policies. Facility opening costs $\{\opencost_i\}$
  are drawn i.i.d.\ from $\texttt{Exponential}(\sfrac{1}{50})$.}
    \label{table:numerical synthetic ratio ExpDist(1/50)}
    \begin{tabular}[t]{cccccc}
    \toprule
    & 
    \CFAlg(1) & \CFAlg(0.7) & \CFAlg(0.5) &
    \CFAlg(0.3) & \CFAlg(0) 
     \\
     \midrule
     uniform $\{\flowi\}$ 
     & 1.022 & 1.008 & 1.011 & 1.024 & 1.049 \\
     dist.-discounted $\{\flowi\}$
     & 1.029 & 1.008 & 1.011 & 1.022 & 1.044 \\
    \bottomrule
    \\
    \toprule
    & 
    \CFAlgP(1) & \CFAlgP(0.7) & \CFAlgP(0.5) &
    \CFAlgP(0.3) & \CFAlgP(0) 
     \\
     \midrule
     uniform $\{\flowi\}$ 
     & 1.001 & 1.002 & 1.009 & 1.023 & 1.049 \\
     dist.-discounted $\{\flowi\}$
     & 1.001 & 1.002 & 1.009 & 1.021 & 1.044 \\
    \bottomrule\\
     \addlinespace[-\aboverulesep] 
    \cmidrule[\heavyrulewidth]{1-3}
    & 
    \GDH & \GDW
     \\
     \cmidrule{1-3}
     uniform $\{\flowi\}$ 
     & 1.191 & 1.186 \\
     dist.-discounted $\{\flowi\}$
     & 1.193 & 1.192 \\
 \cmidrule[\heavyrulewidth]{1-3}
     \addlinespace[-\belowrulesep] 
    \end{tabular}
\end{table}

\begin{table}[ht]
    \centering
    \caption{The average normalized performance for 
    different policies. Facility opening costs $\{\opencost_i\}$
  are drawn i.i.d.\ from $\texttt{Exponential}(\sfrac{1}{200})$.}
    \label{table:numerical synthetic ratio ExpDist(1/200)}
    \begin{tabular}[t]{cccccc}
    \toprule
    & 
    \CFAlg(1) & \CFAlg(0.7) & \CFAlg(0.5) &
    \CFAlg(0.3) & \CFAlg(0) 
     \\
     \midrule
     uniform $\{\flowi\}$ 
     & 1.009 & 1.006 & 1.013 & 1.024 & 1.046 \\
     dist.-discounted $\{\flowi\}$
     & 1.011 & 1.005 & 1.015 & 1.025 & 1.048 \\
    \bottomrule
    \\
    \toprule
    & 
    \CFAlgP(1) & \CFAlgP(0.7) & \CFAlgP(0.5) &
    \CFAlgP(0.3) & \CFAlgP(0) 
     \\
     \midrule
     uniform $\{\flowi\}$ 
     & 1.0 & 1.004 & 1.012 & 1.024 & 1.046 \\
     dist.-discounted $\{\flowi\}$
     & 1.0 & 1.003 & 1.014 & 1.024 & 1.048 \\
    \bottomrule\\
     \addlinespace[-\aboverulesep] 
    \cmidrule[\heavyrulewidth]{1-3}
    & 
    \GDH & \GDW
     \\
     \cmidrule{1-3}
     uniform $\{\flowi\}$ 
     & 1.107 & 1.11 \\
     dist.-discounted $\{\flowi\}$
     & 1.105 & 1.102 \\
 \cmidrule[\heavyrulewidth]{1-3}
     \addlinespace[-\belowrulesep] 
    \end{tabular}
\end{table}
